# Supplementary material for: An Attention-based Weakly Supervised framework for Spitzoid Melanocytic Lesion Diagnosis in WSI
Source: arXiv:2104.09878 source file (2021-04-20)
Supplement: Supplementary file 1 [file Appendix.tex]

\section{Appendix} \label{sec:Appendix}

% ------------------------------ STATIC PROTOTYPES ------------------------------ %

\begin{algorithm}
\caption{Static prototype-based learning strategy.}
\label{static_prototype}
%\footnotesize
%\small
\BlankLine
\KwData{Training $\tau=\{(I_1,y_{I_1}), ..., (I_i,y_{I_i}), ..., (I_{P^\tau},y_{I_{P^\tau}})\}$ and validation $\nu=\{(V_1,y_{V_1}), ..., (V_i,y_{V_i}) , ..., (V_{P^\nu},y_{V_{P^\nu}})\}$ sets.}
\KwResult{\\
\textit{Online stage} $\leftarrow$ Trained base encoder network $\Psi_\phi$ \;
\textit{Offline stage} $\leftarrow$ Inferred prototypes $\rho_c$ \;
\textit{Prediction stage} $\leftarrow$ Predicted labels $\hat{y}_i$ from each $V_i \in \nu$.}
\BlankLine
\textbf{Algorithm:} \\
\textit{Online stage: }\\
\For{$ e \leftarrow 1$ \KwTo $\mathbf \epsilon$}{
    $\phi \leftarrow $ random\;
    \For{$ i \leftarrow 1$ \KwTo $\mathbf P^{\tau}$}{
        $R_i^{\tau} \leftarrow \Psi_{\phi}(I_i)$ \;
        $Z_i \leftarrow \Upsilon_{\phi}(R_i^{\tau})$ \;
        $\hat{y}_i \leftarrow$ softmax$(Z_i)$ \;
    }
    $\mathcal{L}_e(y,\hat{y}) \leftarrow -\sum_{i}{y_i~log(\hat{y_i})}$ \;
    Update $\phi$ using $\nabla_\phi \mathcal{L}_e$
}
\BlankLine
\textit{Offline stage:} \\
\For{$ c \leftarrow 1$ \KwTo $\mathbf 3$}{
    $\rho_c \leftarrow \frac{1}{P^{\tau}}{\sum_{i=1}^{P^{\tau}}{\Psi_{\phi}(I_i)}}, $ where $\phi$ is frozen \;
}
\BlankLine
\textit{Prediction phase: }\\
\For{$ i \leftarrow 1$ \KwTo $\mathbf P^{\nu}$}{
    $R_i^{\nu} \leftarrow \Psi_{\phi}(V_i)$ \;
    \For{$ c \leftarrow 1$ \KwTo $\mathbf 3$}{
        $\delta_{i,c} \leftarrow \sqrt{(\rho_c-R_i^{\nu})^2} $ \;
        $p_{i,c} \leftarrow \frac{\exp{(-\delta_{c,i})}}{\sum_{c'}{\exp{(-\delta_{c',i})}}} $ \;
    }
    $\hat{y}_i \leftarrow argmax(p_{i,c})$
}
\end{algorithm}

% ------------------------------ DYNAMIC PROTOTYPES ------------------------------ %
%% Algorithm
\begin{algorithm}[h]
\caption{Dynamic prototype-based learning strategy.}
\label{dynamic_prototype}
%\footnotesize
%\small
\BlankLine
\KwData{Training $\tau=\{(I_1,y_{I_1}), ..., (I_{P^\tau},y_{I_{P^\tau}})\}$ and validation $\nu=\{(V_1,y_{V_1}), ..., (V_{P^\nu},y_{V_{P^\nu}})\}$ sets.}
\KwResult{\\
Training stage $\leftarrow$ Trained base encoderTrained prototypes $\rho_c$ and predictions $\hat{y}_i$ from each $V_i \in \nu$.}
\BlankLine
\textit{Online stage: }\\
\For{$ e \leftarrow 1$ \KwTo $\mathbf \epsilon$}{
    $\phi \leftarrow $ random\;
    \For{$ i \leftarrow 1$ \KwTo $\mathbf P^{\tau}$}{
        $R_i^{\tau} \leftarrow \Psi_{\phi}(I_i^{\tau})$ \;
        $Z_i \leftarrow \Upsilon_{\phi}(R_i^{\tau})$ \;
        $\hat{y}_i \leftarrow$ softmax$(Z_i)$ \;
    }
    $\mathcal{L}_e(y,\hat{y}) \leftarrow -\sum_{i}{y_i~log(\hat{y_i})}$ \;
    Update $\phi$ using $\nabla_\phi \mathcal{L}_e$
}
\BlankLine
\textit{Offline stage:} \\
\For{$ c \leftarrow 1$ \KwTo $\mathbf 3$}{
    $\rho_c \leftarrow \frac{1}{P}{\sum_{i=1}^{P}{\Psi_{\phi}(I_i^{\tau})}}, $ where $\phi$ is frozen \;
}
\BlankLine
\textit{Prediction phase: }\\
\For{$ i \leftarrow 1$ \KwTo $\mathbf P^{\nu}$}{
    $R_i^{\nu} \leftarrow \Psi_{\phi}(I_i^{\nu})$ \;
    \For{$ c \leftarrow 1$ \KwTo $\mathbf 3$}{
        $\delta_{i,c} \leftarrow \sqrt{(\rho_c-R_i^{\nu})^2} $ \;
        $p_{i,c} \leftarrow \frac{\exp{(-\delta_{c,i})}}{\sum_{c'}{\exp{(-\delta_{c',i})}}} $ \;
    }
    $\hat{y}_i \leftarrow argmax(p_{i,c})$
}
\end{algorithm}
